# Supplementary material for: Human-Level Accuracy, Non-Human Strategies: Revealing Model-Human Divergence in Video Physical Reasoning
Source: arXiv:2609.22788 source file (2026-09-19)
Supplement: Supplementary file 1 [file supplementary.tex]

\documentclass[runningheads]{llncs}

% ---------------------------------------------------------------
% ECCV package (same as main)
% Camera-ready supplementary material mode.
\usepackage{eccv}

% ---------------------------------------------------------------
% Standard packages
\usepackage{eccvabbrv}
\usepackage{graphicx}
\usepackage{booktabs}

% Additional packages
\usepackage{multirow}
\usepackage{float}
\usepackage{amsmath,amssymb}
\usepackage{dsfont}
\usepackage{xcolor}

% Hyperref
\usepackage{hyperref}

% ORCID
\usepackage{orcidlink}

% ---------------------------------------------------------------
% Custom commands (same as main)
\newcommand{\vjepa}{V-JEPA2}
\newcommand{\vmae}{VideoMAEv2}
\newcommand{\dino}{DINOv2}
\newcommand{\rvm}{RVM}

% ---------------------------------------------------------------
\begin{document}

\title{Supplementary Material:\\Human-Level Accuracy, Non-Human Strategies}

\titlerunning{Supplementary Material}

\author{Fanhong Li\inst{1} \and
Shurui Zheng\inst{1} \and
Zi Yin\inst{1} \and
Junbo Cui\inst{2} \and
Lei Ji\inst{3} \and
Jia Liu\inst{1}\thanks{Corresponding author.}}

\authorrunning{F.~Li \etal}

\institute{
Tsinghua University, Beijing, China\\
\email{\{lifh21,zhengsr23,z-yin21\}@mails.tsinghua.edu.cn, liujiaTHU@tsinghua.edu.cn}
\and
ModelBest Inc., Beijing, China\\
\email{cuijb2000@gmail.com}
\and
Microsoft, Beijing, China\\
\email{leiji@microsoft.com}
}

\maketitle

\appendix
\input{sec_appendix}

\clearpage
\bibliographystyle{splncs04}
\bibliography{main}

\end{document}
